# Supplementary material for: THRONE: An Object-based Hallucination Benchmark for the Free-form Generations of Large Vision-Language Models
Source: arXiv:2405.05256 source file (2025-04-03)
Supplement: Supplementary file 1 [file 01-model_details.tex]

\cvprsection{Evaluated LVLM Details}\label{smsec:model_details}
In this section, we briefly outline details in the LVLMs we evaluate with \throne, such as design choices and training data.

\paragraph*{LLaMA-Adapter-v2}~\cite{gao2023llamaadapter} \\
\begin{itemize}
    \item LLM:\@ LLaMA-v1-7b~\cite{touvron2023llama}
    \item Image Encoder: CLIP ViT-L/14~\cite{radford2021learning}
    \item Vision-Language Connector: Linear projection, learnt visual queries and additional vision transformer blocks 
    \item Pretraining Data:
    LAION-400M~\cite{schuhmann2021laion},
    COYO-700M~\cite{kakaobrain2022coyo-700m},
    MMC4~\cite{zhu2023multimodal},
    SBU~\cite{NIPS2011_5dd9db5e},
    CC3M~\cite{sharma2018conceptual},
    and COCO Captions~\cite{fang2015captions}
    \item Finetuning Data:
    GPT4LLM~\cite{peng2023instruction} and
    LLaVA~\cite{liu2023visual}
\end{itemize}

\paragraph*{LLaMA-Adapter-v2.1}~\cite{gao2023llamaadapter} \\
Same as LLaMA-Adapter-v2 with one modification.
\begin{itemize}
    \item Finetuning Data:
    GPT4LLM~\cite{peng2023instruction},
    LLaVA~\cite{liu2023visual} \emph{and
    VQAv2}~\cite{antol2015vqa}
\end{itemize}

\paragraph*{InstructBLIP}~\cite{dai2023instructblip} \\
\begin{itemize}
    \item LLM:\@ Vicuna-v1.1-7b~\cite{chiang2023vicuna}
    \item Image Encoder: EVA ViT-g/14~\cite{fang2023eva}
    \item Visual-Language Connector: Querying Transformer (Q-Former)
    \item Pretraining Data:
    LAION400M~\cite{schuhmann2021laion},
    CC3M~\cite{sharma2018conceptual},
    CC12M~\cite{changpinyo2021conceptual},
    Visual Genome~\cite{krishna2017visual}
    and COCO Captions~\cite{fang2015captions}
    \item Finetuning Data:
    COCO Captions~\cite{fang2015captions},
    TextCaps~\cite{sidorov2019textcaps},
    VQAv2~\cite{antol2015vqa},
    OKVQA~\cite{okvqa},
    A-OKVQA~\cite{AOKVQA},
    OCR-VQA~\cite{8978122} and
    LLaVA~\cite{liu2023visual}
\end{itemize}

\paragraph*{Otter-Image}~\cite{li2023otter} \\
\begin{itemize}
    \item LLM:\@ MPT-7b~\cite{mosaicml2023mpt} (initialized from OpenFlamingo weights~\cite{anas_awadalla_2023_7733589})
    \item Image Encoder: CLIP ViT-L/14~\cite{radford2021learning}
    \item Visual-Language Connector: Cross-attention modules between visual and language features
    \item Pretraining Data:
    MMC4~\cite{zhu2023multimodal},
    LAION-2B-en~\cite{schuhmann2022laion}
    and synthetic data from ChatGPT~\cite{openai2023chatgpt} 
    \item Finetuning Data: MIMIC-IT~\cite{li2023otter}
\end{itemize}

\paragraph*{MiniGPT-4}~\cite{zhu2023minigpt} \\
\begin{itemize}
    \item LLM:\@ Vicuna-v0-7b~\cite{chiang2023vicuna}
    \item Image Encoder: EVA ViT-g/14~\cite{fang2023eva}
    \item Vision-Language Connector: Linear projection and Q-Former (initialized and frozen from BLIP-2~\cite{li2023blip2})
    \item Pretraining Data:
    CC3M~\cite{sharma2018conceptual},
    CC12M~\cite{changpinyo2021conceptual},
    SBU~\cite{NIPS2011_5dd9db5e} and
    LAION-400M~\cite{schuhmann2021laion}
    \item Finetuning Data:
    Synthetic data using ChatGPT~\cite{openai2023chatgpt}
    and a sample of CC3M/CC12M images~\cite{changpinyo2021conceptual,sharma2018conceptual}
\end{itemize}

\paragraph*{MiniGPT-v2}~\cite{chen2023minigpt2} \\
\begin{itemize}
    \item LLM:\@ Llama2-7b-chat~\cite{touvron2023llama2}
    \item Image Encoder: EVA ViT-g/14~\cite{fang2023eva}
    \item Vision-Language Connector: Linear projection
    \item Pretraining Data:
    GRiT-20M~\cite{peng2023kosmos2},
    COCO Captions~\cite{fang2015captions},
    TextCaps~\cite{sidorov2019textcaps},
    RefCOCO/+/g~\cite{kazemzadeh2014referitgame,mao2016generation},
    Visual Genome~\cite{krishna2017visual},
    GQA~\cite{hudson2019gqa},
    VQAv2~\cite{antol2015vqa},
    OKVQA~\cite{okvqa},
    A-OKVQA~\cite{AOKVQA} and
    OCR-VQA~\cite{8978122}
    \item Finetuning Data:
    COCO Captions~\cite{fang2015captions},
    TextCaps~\cite{sidorov2019textcaps},
    RefCOCO/+/g~\cite{kazemzadeh2014referitgame,mao2016generation},
    Visual Genome~\cite{krishna2017visual},
    GQA~\cite{hudson2019gqa},
    VQAv2~\cite{antol2015vqa},
    OKVQA~\cite{okvqa},
    A-OKVQA~\cite{AOKVQA},
    LLaVA~\cite{liu2023visual},
    Flickr30k~\cite{plummer2015flickr30k} and
    LLaVA~\cite{liu2023visual}
\end{itemize}

\paragraph*{Qwen-VL-Chat}~\cite{Qwen-VL} \\
\begin{itemize}
    \item LLM:\@ Qwen-LM~\cite{bai2023qwen}
    \item Image Encoder: OpenCLIP ViT-g~\cite{ilharco_gabriel_2021_5143773}
    \item Vision-Language Connector: Single cross-attention block between image features and learnt visual queries 
    \item Pretraining Data:
    LAION-2B-en~\cite{schuhmann2022laion},
    COYO-700M~\cite{kakaobrain2022coyo-700m},
    CC3M~\cite{sharma2018conceptual},
    CC12M~\cite{changpinyo2021conceptual},
    SBU~\cite{NIPS2011_5dd9db5e},
    COCO Caption~\cite{fang2015captions}
    and DataComp~\cite{gadre2023datacomp}
    \item Finetuning Data:
    LAION-2B-en/zh~\cite{schuhmann2022laion},
    COYO-700M~\cite{kakaobrain2022coyo-700m},
    CC3M~\cite{sharma2018conceptual},
    CC12M~\cite{changpinyo2021conceptual},
    SBU~\cite{NIPS2011_5dd9db5e},
    DataComp~\cite{gadre2023datacomp},
    COCO Caption~\cite{fang2015captions},
    GQA~\cite{hudson2019gqa},
    Visual Genome~\cite{krishna2017visual},
    VQAv2~\cite{antol2015vqa},
    DVQA~\cite{kafle2018dvqa},
    OCR-VQA~\cite{8978122},
    DocVQA~\cite{mathew2021docvqa},
    TextVQA~\cite{singh2019towards},
    ChartQA~\cite{masry-etal-2022-chartqa},
    AI2D~\cite{kembhavi2016diagram},
    GRiT~\cite{peng2023kosmos2},
    VisualGenome~\cite{krishna2017visual},
    RefCOCO/+/g~\cite{kazemzadeh2014referitgame,mao2016generation},
    Synthetic OCR data,
    Common Crawl PDF~\cite{ccpdf}
\end{itemize}

\paragraph*{mPLUG-Owl}~\cite{ye2023mplug}
\begin{itemize}
    \item LLM:\@ LLaMA-7b~\cite{touvron2023llama}
    \item Image Encoder: CLIP ViT-L/14~\cite{radford2021learning}
    \item Vision-Language Connector: Cross-attention and learnt visual queries
    \item Pretraining Data:
    LAION-400M~\cite{schuhmann2021laion},
    COYO-700M~\cite{kakaobrain2022coyo-700m},
    CC3M~\cite{sharma2018conceptual} and
    COCO Captions~\cite{fang2015captions}
    \item Finetuning Data:
    LLaVA~\cite{liu2023visual},
    Alpaca~\cite{alpaca},
    Vicuna~\cite{chiang2023vicuna}
    and Baize~\cite{xu2023baize}
\end{itemize}

\paragraph*{LRV-Instruction-v2}~\cite{liu2023aligning} \\
Same as mPLUG-Owl with one modification.
\begin{itemize}
    \item Finetuning Data:
    LRV-Instruction-v2~\cite{liu2023aligning},
    Alpaca~\cite{alpaca},
    Vicuna~\cite{chiang2023vicuna}
    and Baize~\cite{xu2023baize}
\end{itemize}

\paragraph*{LLaVA-v1.3}~\cite{liu2023visual} \\
\begin{itemize}
    \item LLM:\@ Vicuna-v1.3-7b~\cite{chiang2023vicuna}
    \item Image Encoder: CLIP ViT-L/14~\cite{radford2021learning}
    \item Pretraining Data:
    LAION-400M~\cite{schuhmann2021laion},
    CC3M~\cite{sharma2018conceptual} and
    SBU~\cite{NIPS2011_5dd9db5e}
    \item Finetuning Data:
    LLaVA~\cite{liu2023visual}
\end{itemize}

\paragraph*{LLaVA-v1.5}~\cite{liu2023improved} \\
\begin{itemize}
\item LLM:\@ Vicuna-v1.5-7b~\cite{chiang2023vicuna}
\item Image Encoder: CLIP ViT-L/14~\cite{radford2021learning}
\item Pretraining Data:
LAION-400M~\cite{schuhmann2021laion},
CC3M~\cite{sharma2018conceptual} and
SBU~\cite{NIPS2011_5dd9db5e}
\item Finetuning Data:
LLaVA~\cite{liu2023visual},
VQAv2~\cite{antol2015vqa},
GQA~\cite{hudson2019gqa},
TextVQA~\cite{singh2019towards},
OCR-VQA~\cite{8978122}
and VisualGenome~\cite{krishna2017visual}
\end{itemize}
