# Supplementary material for: THRONE: An Object-based Hallucination Benchmark for the Free-form Generations of Large Vision-Language Models
Source: arXiv:2405.05256 source file (2025-04-03)
Supplement: Supplementary file 3 [file preamble.tex]

%
% --- inline annotations
%
\usepackage{booktabs}
\usepackage[table,xcdraw,dvipsnames]{xcolor}
\usepackage{multirow}
\usepackage{lipsum}
\usepackage{adjustbox}
\usepackage{colortbl}
\usepackage{amssymb}
\usepackage{pifont}
% \usepackage[pagebackref,breaklinks,colorlinks]{hyperref}
% \usepackage[numbers,sort]{natbib}
% \usepackage[dvipsnames]{xcolor}
% \linespread{2.0}
\usepackage{xspace}

\newcommand{\red}[1]{{\color{red}#1}}
\newcommand{\todo}[1]{{\color{red}#1}}
\newcommand{\TODO}[1]{\textbf{\color{red}[TODO:\@ #1]}}
\newcommand{\best}[1]{{\color[HTML]{3531FF}{\textbf{#1}}}}
\newcommand{\sbest}[1]{{\color[HTML]{FE0000}{\textit{#1}}}}
% --- disable by uncommenting  
% \renewcommand{\TODO}[1]{}
% \renewcommand{\todo}[1]{#1}

\newcommand{\prannay}[1]{{\textcolor{red}{Prannay: #1} }}
\newcommand{\zhizhong}[1]{{\textcolor{blue}{Zhizhong: #1} }}
\newcommand{\hao}[1]{{\textcolor{magenta}{Hao: #1} }}
\newcommand{\yoni}[1]{{\textcolor{olive}{Yoni: #1} }}
\newcommand{\redact}[1]{{\textcolor{red}{Removing: #1} }}
\newcommand{\throne}{\textsc{THR\={O}NE}\xspace}

% % uncomment to blank all author comments
% \renewcommand{\prannay}[1]{}
% \renewcommand{\zhizhong}[1]{}
% \renewcommand{\hao}[1]{}
% \renewcommand{\yoni}[1]{}


\newcommand\blfootnote[1]{%
  \begingroup
  \renewcommand\thefootnote{}\footnote{#1}%
  \addtocounter{footnote}{-1}%
  \endgroup
}
\newcommand{\xmark}{\ding{55}}%
\newcommand{\texttts}[1]{\texttt{\footnotesize #1}}
